# Supplementary material for: Energy-based Potential Games for Joint Motion Forecasting and Control
Source: arXiv:2312.01811 source file (2023-12-04)

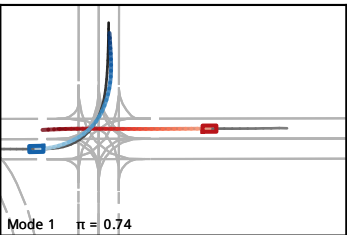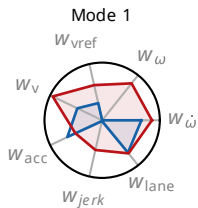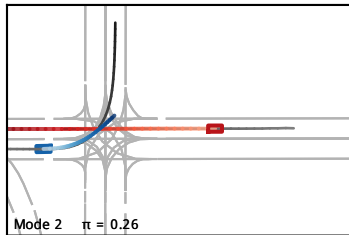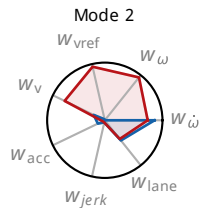





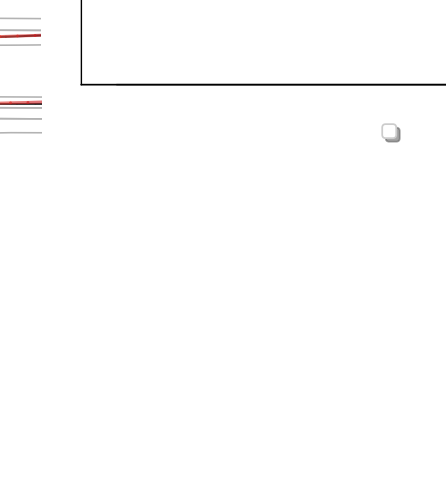

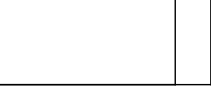

Supplement: Supplementary file 1 [file col_qual_fig_suppl.pdf]
